# Supplementary material for: A Novel NPT Thermodynamic Integration Scheme to Derive Rigorous Gibbs Free Energies for Crystalline Solids
Source: arXiv:2602.20738 ancillary file (2026-02-24)
Supplement: Supplementary file 1 [file SI_1_to_5.pdf]

# A Novel NPT Thermodynamic Integration Scheme to Derive Rigorous Gibbs Free Energies for Crystalline Solids

Karel L. K. De Witte, Tom Braeckevelt, Massimo Bocus, Sander Vandenhaute, and Veronique Van Speybroeck*

*Center for Molecular Modeling, Ghent University, 9052 Zwijnaarde, Belgium*

E-mail: Veronique.VanSpeybroeck@UGent.be

# 1 Helmholtz free energy of the NVT harmonic approximation of a crystal

In this section, we derive the Helmholtz free energy of a crystalline solid within the harmonic approximation. The system consists of $N$ atoms at temperature $T$ and volume $V$. Although this derivation is known in the literature,[1] it is included here for completeness and because it is instructive for understanding the methodology introduced in the main text.

**Hamiltonian and harmonic approximation** The classical Hamiltonian in Cartesian coordinates $\mathbf{r}$ and conjugate momenta $\mathbf{p}$ is given by

$$H(\mathbf{r},\mathbf{p}) = \frac{1}{2}\,\mathbf{p}\cdot\mathbf{M}^{-1}\cdot\mathbf{p}^{T} + U(\mathbf{r}), \tag{1}$$

where

$$\mathbf{r} = \begin{bmatrix} r_{1x} & r_{1y} & \cdots & r_{Nz} \end{bmatrix}, \qquad \mathbf{p} = \begin{bmatrix} p_{1x} & p_{1y} & \cdots & p_{Nz} \end{bmatrix}. \tag{2}$$

The mass matrix $\mathbf{M}$ is diagonal and reads

$$\mathbf{M} = \begin{bmatrix} m_1 & 0 & 0 & 0 & \cdots & 0 \\ 0 & m_1 & 0 & 0 & \cdots & 0 \\ 0 & 0 & m_1 & 0 & \cdots & 0 \\ 0 & 0 & 0 & m_2 & \cdots & 0 \\ \vdots & \vdots & \vdots & \vdots & \ddots & \vdots \\ 0 & 0 & 0 & 0 & \cdots & m_N \end{bmatrix}, \tag{3}$$

where each atomic mass appears three times, corresponding to the three Cartesian directions.

We expand the potential energy $U(\mathbf{r})$ in a Taylor series around a reference configuration

$\mathbf{r}_0$:

$$U(\mathbf{r}) = U(\mathbf{r}_0) + \nabla U(\mathbf{r}_0) \cdot (\mathbf{r} - \mathbf{r}_0)^T \\ + \frac{1}{2}(\mathbf{r} - \mathbf{r}_0) \cdot \mathbf{H}(\mathbf{r}_0) \cdot (\mathbf{r} - \mathbf{r}_0)^T + \mathcal{O}(|\mathbf{r} - \mathbf{r}_0|^3), \tag{4}$$

where the Hessian matrix $\mathbf{H}$ is defined as

$$\mathbf{H}_{ij} = \frac{\partial^2 U}{\partial r_i \partial r_j}. \tag{5}$$

Choosing $\mathbf{r}_0$ to be a minimum of $U(\mathbf{r})$ implies $\nabla U(\mathbf{r}_0) = 0$. Retaining terms up to second-order yields the harmonic Hamiltonian

$$H(\mathbf{r}, \mathbf{p}) = E_0 + \frac{1}{2}\mathbf{p} \cdot \mathbf{M}^{-1} \cdot \mathbf{p}^T + \frac{1}{2}(\mathbf{r} - \mathbf{r}_0) \cdot \mathbf{H}(\mathbf{r}_0) \cdot (\mathbf{r} - \mathbf{r}_0)^T, \tag{6}$$

where $E_0 = U(\mathbf{r}_0)$.

**Mass-weighted coordinates** We introduce mass-weighted coordinates and momenta via the transformation

$$\begin{cases} \mathbf{s} = \mathbf{p} \cdot \mathbf{M}^{-1/2}, \\ \mathbf{q} = (\mathbf{r} - \mathbf{r}_0) \cdot \mathbf{M}^{1/2}. \end{cases} \tag{7}$$

This transformation is canonical, as can be verified using the symplectic condition.

In these variables, the Hamiltonian becomes

$$H(\mathbf{q}, \mathbf{s}) = E_0 + \frac{1}{2}\mathbf{s} \cdot \mathbf{s}^T + \frac{1}{2}\mathbf{q} \cdot \mathbf{M}^{-1/2}\mathbf{H}\mathbf{M}^{-1/2} \cdot \mathbf{q}^T. \tag{8}$$

The mass-weighted Hessian

$$\mathbf{M}^{-1/2}\mathbf{H}\mathbf{M}^{-1/2} \tag{9}$$

is real and symmetric, and can therefore be diagonalized:

$$\mathbf{M}^{-1/2}\mathbf{H}\mathbf{M}^{-1/2} = \mathbf{N}^T\mathbf{D}\mathbf{N}, \tag{10}$$

where $\mathbf{N}$ is orthogonal,

$$\mathbf{N}^T\mathbf{N} = \mathbf{N}\mathbf{N}^T = \mathbf{I}, \tag{11}$$

and $\mathbf{D}$ is diagonal with elements $\omega_i^2$,

$$\mathbf{D} = \mathrm{diag}(\omega_1^2, \omega_2^2, \ldots, \omega_{3N}^2). \tag{12}$$

**Normal modes** We perform a second canonical transformation to normal-mode coordinates:

$$\begin{cases} \mathbf{k} = \mathbf{s} \cdot \mathbf{N}, \\ \mathbf{x} = \mathbf{q} \cdot \mathbf{N}^T. \end{cases} \tag{13}$$

The Hamiltonian is then decoupled into a sum of independent harmonic oscillators,

$$H(\mathbf{x}, \mathbf{k}) = E_0 + \frac{1}{2}\mathbf{k} \cdot \mathbf{k}^T + \frac{1}{2}\mathbf{x} \cdot \mathbf{D} \cdot \mathbf{x}^T = E_0 + \sum_{i=1}^{3N} \left( \frac{k_i^2}{2} + \frac{1}{2}\omega_i^2 x_i^2 \right). \tag{14}$$

**Partition function** The classical canonical partition function is

$$Z = \frac{1}{h^{3N}} \int \mathrm{d}^{3N}\mathbf{k} \int \mathrm{d}^{3N}\mathbf{x} \, \exp\left[-\beta H(\mathbf{x}, \mathbf{k})\right], \tag{15}$$

where $\beta = (k_\mathrm{B}T)^{-1}$.

For a crystal, three eigenvalues $\omega_i$ vanish due to translational invariance, and the corresponding modes are excluded from the vibrational partition function. The contribution of the translational degrees of freedom yields a factor $V/\lambda^3$, where $V$ is the volume and $\lambda = \frac{h}{\sqrt{2\pi M k_\mathrm{B} T}}$ is the thermal wavelength of the center of mass with $M$ the total mass of the system. For macroscopic systems, this contribution is negligible and is omitted here.

The integrals factorize into one-dimensional Gaussian integrals, yielding

$$Z = e^{-\beta E_0} \prod_{i=1}^{3N-3} \frac{1}{\beta\hbar\omega_i}. \tag{16}$$

**Helmholtz free energy** The Helmholtz free energy in the harmonic approximation is therefore

$$F_{\mathrm{harm}} = -k_{\mathrm{B}}T \ln Z = E_0 + k_{\mathrm{B}}T \sum_{i=1}^{3N-3} \ln\left(\frac{\hbar\omega_i}{k_{\mathrm{B}}T}\right). \qquad (17)$$

# 2 Implementation of the novel NPT TI scheme

This section introduces: (i) the construction of the extended Hessian, and the calculation of $G_{\text{ref}}$, and (ii) the computation of forces and stresses from the NPT harmonic PES. All the developed code is available on the following Zenodo repository: 10.5281/zenodo.18632301.

## 2.1 Extended Hessian

The extended Hessian $\mathbf{H}_{\text{ext}}$ of the function $U_f$ quantifies the local curvature of $U_f$ at the minimum $(\mathbf{d}_{i,0}, \mathbf{h}_0)$. For an $N$-particle system, $\mathbf{H}_{\text{ext}}$ is a $(3N+9) \times (3N+9)$ matrix, because each atom contributes three deformed coordinates and the cell contributes nine Cartesian degrees of freedom. Its structure is

$$\mathbf{H}_{\text{ext}} = \begin{bmatrix} \frac{\partial^2 U_f}{\partial \mathbf{d} \partial \mathbf{d}} & \frac{\partial^2 U_f}{\partial \mathbf{d} \partial \mathbf{h}} \\ \frac{\partial^2 U_f}{\partial \mathbf{h} \partial \mathbf{d}} & \frac{\partial^2 U_f}{\partial \mathbf{h} \partial \mathbf{h}} \end{bmatrix} = \begin{bmatrix} \nabla_{\mathbf{d}} \otimes \nabla_{\mathbf{d}} U_f & \nabla_{\mathbf{d}} \otimes \nabla_{\mathbf{h}} U_f \\ \nabla_{\mathbf{h}} \otimes \nabla_{\mathbf{d}} U_f & \nabla_{\mathbf{h}} \otimes \nabla_{\mathbf{h}} U_f \end{bmatrix} \tag{18}$$

or more explicitly:

$$\mathbf{H}_{\text{ext}} = \begin{bmatrix} \frac{\partial^2 U_f}{\partial d_{1x}^2} & \frac{\partial^2 U_f}{\partial d_{1x} \partial d_{1y}} & \cdots & \frac{\partial^2 U_f}{\partial d_{1x} \partial d_{Nz}} & \frac{\partial^2 U_f}{\partial d_{1x} \partial h_{11}} & \cdots & \frac{\partial^2 U_f}{\partial d_{1x} \partial h_{33}} \\ \frac{\partial^2 U_f}{\partial d_{1y} \partial d_{1x}} & \frac{\partial^2 U_f}{\partial d_{1y}^2} & \cdots & \frac{\partial^2 U_f}{\partial d_{1y} \partial d_{Nz}} & \frac{\partial^2 U_f}{\partial d_{1y} \partial h_{11}} & \cdots & \frac{\partial^2 U_f}{\partial d_{1y} \partial h_{33}} \\ \vdots & \vdots & \ddots & \vdots & \vdots & \ddots & \vdots \\ \frac{\partial^2 U_f}{\partial d_{Nz} \partial d_{1x}} & \frac{\partial^2 U_f}{\partial d_{Nz} \partial d_{1y}} & \cdots & \frac{\partial^2 U_f}{\partial d_{Nz}^2} & \frac{\partial^2 U_f}{\partial d_{Nz} \partial h_{11}} & \cdots & \frac{\partial^2 U_f}{\partial d_{Nz} \partial h_{33}} \\ \frac{\partial^2 U_f}{\partial h_{11} \partial d_{1x}} & \frac{\partial^2 U_f}{\partial h_{11} \partial d_{1y}} & \cdots & \frac{\partial^2 U_f}{\partial h_{11} \partial d_{Nz}} & \frac{\partial^2 U_f}{\partial h_{11}^2} & \cdots & \frac{\partial^2 U_f}{\partial h_{11} \partial h_{33}} \\ \vdots & \vdots & \ddots & \vdots & \vdots & \ddots & \vdots \\ \frac{\partial^2 U_f}{\partial h_{33} \partial d_{1x}} & \frac{\partial^2 U_f}{\partial h_{33} \partial d_{1y}} & \cdots & \frac{\partial^2 U_f}{\partial h_{33} \partial d_{Nz}} & \frac{\partial^2 U_f}{\partial h_{33} \partial h_{11}} & \cdots & \frac{\partial^2 U_f}{\partial h_{33}^2} \end{bmatrix}. \tag{19}$$

The first step is to determine the minimum $(\mathbf{d}_{i,0}, \mathbf{h}_0)$ of

$$U_f = U_{\text{real}} + U_{\text{bias}}, \qquad U_{\text{bias}} = PV - \frac{N-2}{\beta} \ln V.$$

We perform a full geometry optimization of the system using the Atomic Simulation Environment (ASE).[2] Both the atomic coordinates as well as the cell vectors are relaxed, such that all atomic forces and cell stresses vanish once a stationary point is found. The real PES $U_{\text{real}}$ is represented by a MACE MLIP,[3] while the bias PES is implemented in PLUMED.[4] The extended Hessian is then evaluated at this optimized configuration.

Figure 1 summarizes the workflow for constructing the extended Hessian. The matrix is assembled row by row. For each row, two perturbed geometries are generated: one with a positive perturbation of a chosen coordinate and one with the corresponding negative perturbation. Each perturbed geometry yields forces and stresses, which are converted into first-order derivatives of the energy using the appropriate Jacobian transformations. These first-order derivatives are then combined using central finite-difference expressions to obtain the corresponding second-order derivative. Note that we compute all extended Hessian matrix elements explicitly. Verifying the symmetry of the matrix afterwards serves as a simple and handy sanity check. Given that symmetry up to high precision was satisfied, the final extended Hessian was computed as $\mathbf{H}_{\text{ext}} = 0.5(\mathbf{H}_{\text{ext}} + \mathbf{H}_{\text{ext}}^T)$.

### 2.1.1 Computing first-order derivatives

First-order derivatives are obtained from the forces and stresses computed by the MACE and PLUMED PES upon energy evaluation. The PLUMED forces and stresses are analytic, while the MACE contributions are obtained via automatic differentiation and are therefore semi-analytic.[5] The force on atom $i$ is related to the gradient of $U_f$ with respect to its Cartesian coordinates $\mathbf{r}_i$ through

$$\mathbf{F}_i = -\nabla_{\mathbf{r}_i} U_f. \tag{20}$$

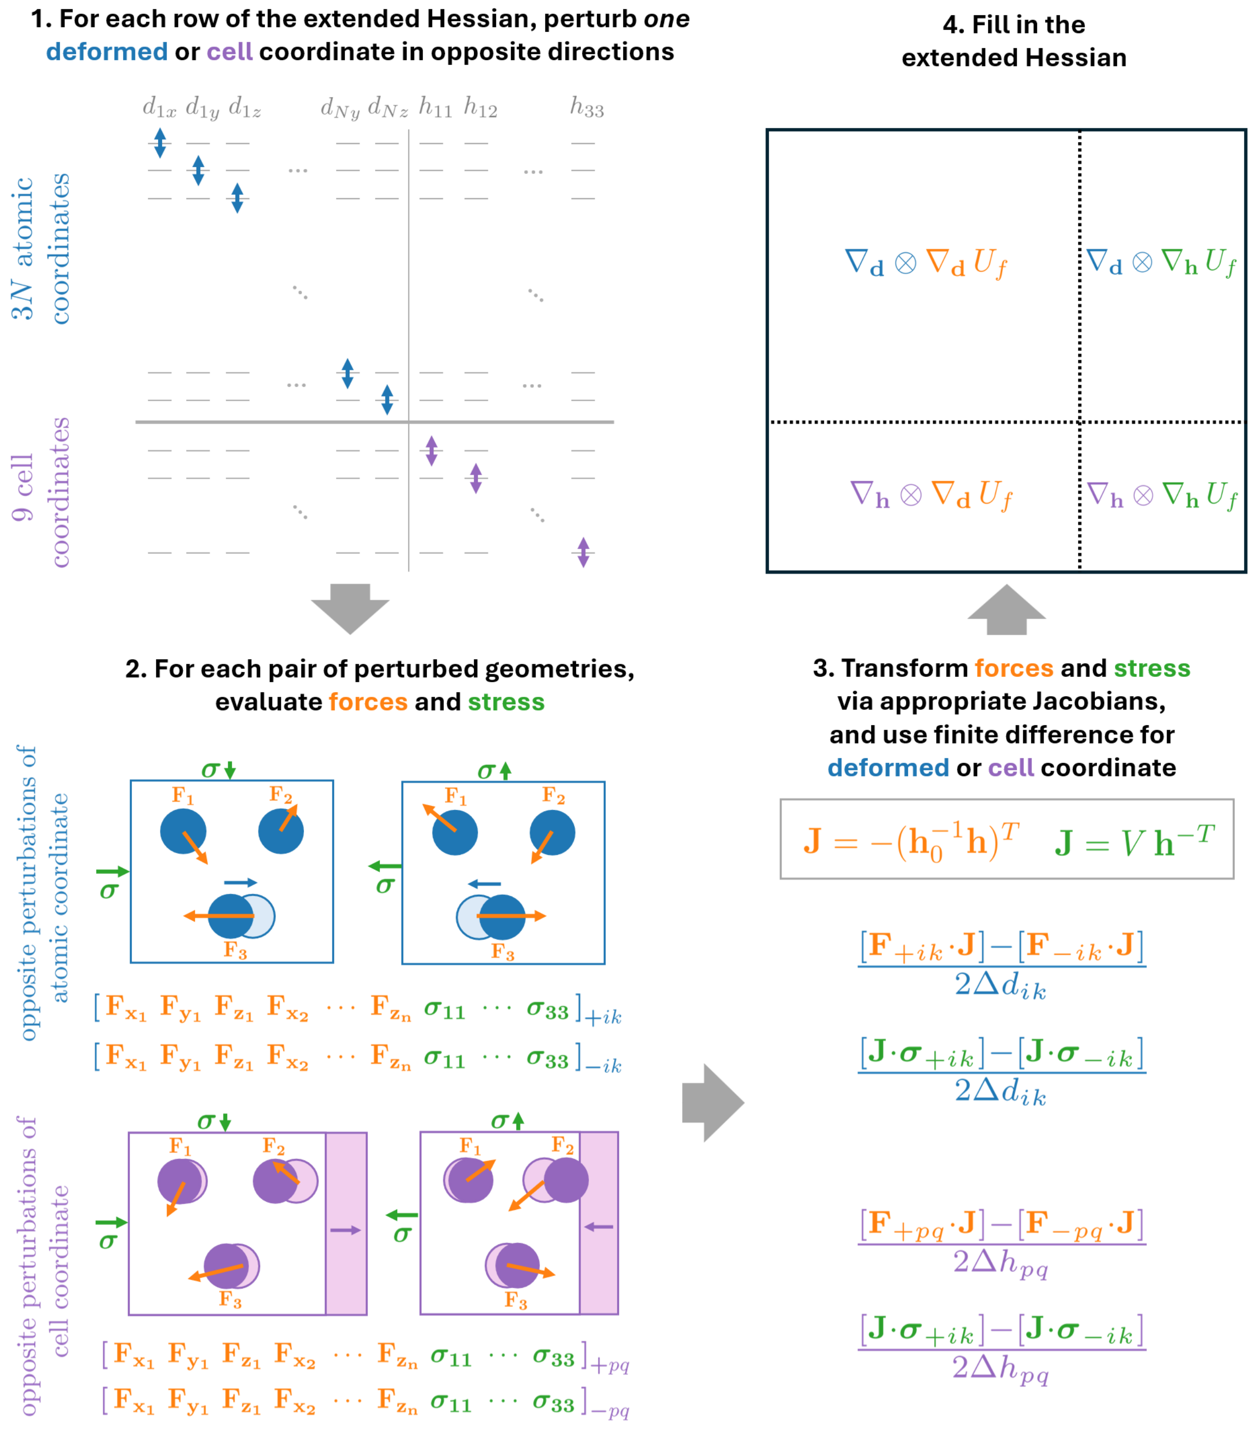


Figure 1: Schematic overview of the numerical construction of the extended Hessian.

The deformed coordinates are defined as

$$\mathbf{d}_i = \mathbf{r}_i \cdot \mathbf{h}^{-1}\mathbf{h}_0, \tag{21}$$

This yields the gradient with respect to deformed coordinates:

$$\nabla_{\mathbf{d}_i} U_f = \nabla_{\mathbf{r}_i} U_f \cdot (\mathbf{h}_0^{-1}\mathbf{h})^T = -\mathbf{F}_i \cdot (\mathbf{h}_0^{-1}\mathbf{h})^T. \tag{22}$$

The stress tensor $\boldsymbol{\sigma}$ is related to the derivative of $U_f$ with respect to strain $\boldsymbol{\varepsilon}$ through:

$$\boldsymbol{\sigma} = \frac{1}{V}\frac{\partial U_f}{\partial \boldsymbol{\varepsilon}}. \tag{23}$$

The stress is further connected to the gradient of the energy with respect to the cell matrix $\mathbf{h}$ via:[6]

$$\boldsymbol{\sigma} = \frac{1}{V}\mathbf{h}^T \frac{\partial U_f}{\partial \mathbf{h}}. \tag{24}$$

This expression allows us to extract the nine cell derivatives required for the construction of the extended Hessian.

### 2.1.2 Second-order derivatives via atomic perturbations

In this section is explained how the block matrices $\nabla_{\mathbf{d}} \otimes \nabla_{\mathbf{d}} U_f$ and $\nabla_{\mathbf{d}} \otimes \nabla_{\mathbf{h}} U_f$ are computed. For each row of these matrices, one deformed coordinate is perturbed both positively and negatively. While forces and stresses provide analytical first-order derivatives, finite differences are used to construct the second-order derivatives.

For row index $3(i-1)+k$, the deformed coordinate $d_{ik}$ is perturbed by a small displacement $\pm\Delta d_{ik}$ ($i = 1, \ldots, N$; $k = 1, 2, 3$ corresponding to $x, y, z$). The positively perturbed geometry (via $+\Delta d_{ik}$) yields a force vector of length $3N$ and a stress tensor written as a row

vector of length 9:

$$
\begin{aligned}
\mathbf{F}_{+ik} &= \begin{bmatrix} F_{1x} & F_{1y} & F_{1z} & F_{2x} & \dots & F_{Nz} \end{bmatrix}_{+ik} \\
\boldsymbol{\sigma}_{+ik} &= \begin{bmatrix} \sigma_{11} & \sigma_{12} & \sigma_{13} & \sigma_{21} & \dots & \sigma_{33} \end{bmatrix}_{+ik}
\end{aligned} \tag{25}
$$

Analogously, the negatively perturbed geometry (via $-\Delta d_{ik}$) yields:

$$
\begin{aligned}
\mathbf{F}_{-ik} &= \begin{bmatrix} F_{1x} & F_{1y} & F_{1z} & F_{2x} & \dots & F_{Nz} \end{bmatrix}_{-ik} \\
\boldsymbol{\sigma}_{-ik} &= \begin{bmatrix} \sigma_{11} & \sigma_{12} & \sigma_{13} & \sigma_{21} & \dots & \sigma_{33} \end{bmatrix}_{-ik}
\end{aligned} \tag{26}
$$

The mixed second derivatives with respect to the deformed coordinates are obtained as:

$$
\begin{aligned}
\frac{\partial^2 U_f}{\partial d_{ik}\,\partial \mathbf{d}} &= \frac{\left[-\mathbf{F}_{+ik} \cdot (\mathbf{h}_0^{-1}\mathbf{h})^T\right] - \left[-\mathbf{F}_{-ik} \cdot (\mathbf{h}_0^{-1}\mathbf{h})^T\right]}{2\Delta d_{ik}} \\
&= \frac{\mathbf{F}_{+ik} - \mathbf{F}_{-ik}}{2\Delta d_{ik}}
\end{aligned} \tag{27}
$$

where $(\mathbf{h}_0^{-1}\mathbf{h})^T = \mathbf{1}$ because a perturbation of a deformed coordinate does not modify the simulation cell and thus $\mathbf{h} = \mathbf{h}_0$.

The mixed second derivatives with respect to deformed and cell coordinates are given by:

$$
\begin{aligned}
\frac{\partial^2 U_f}{\partial d_{ik}\,\partial \mathbf{h}} &= \frac{\left[V\,\mathbf{h}^{-T}\boldsymbol{\sigma}_{+ik}\right] - \left[V\,\mathbf{h}^{-T}\boldsymbol{\sigma}_{-ik}\right]}{2\Delta d_{ik}} \\
&= V\,\mathbf{h}^{-T} \cdot \frac{\boldsymbol{\sigma}_{+ik} - \boldsymbol{\sigma}_{-ik}}{2\Delta d_{ik}}
\end{aligned} \tag{28}
$$

### 2.1.3 Second-order derivatives via cell perturbations

In this section is explained how the block matrices $\nabla_{\mathbf{h}} \otimes \nabla_{\mathbf{d}}\, U_f$ and $\nabla_{\mathbf{h}} \otimes \nabla_{\mathbf{h}}\, U_f$ are computed, analogously to previous section.

For row index $3N + 3(p-1) + q$, the cell coordinate $h_{pq}$ is perturbed by $\pm\,\Delta h_{pq}$ $(p, q =$

1, 2, 3). The positively perturbed geometry yields:

$$\begin{aligned}\mathbf{F}_{+pq} &= \begin{bmatrix} F_{1x} & F_{1y} & F_{1z} & F_{2x} & \dots & F_{Nz} \end{bmatrix}_{+pq} \\ \boldsymbol{\sigma}_{+pq} &= \begin{bmatrix} \sigma_{11} & \sigma_{12} & \sigma_{13} & \sigma_{21} & \dots & \sigma_{33} \end{bmatrix}_{+pq}\end{aligned} \tag{29}$$

Similarly, the negatively perturbed geometry yields:

$$\begin{aligned}\mathbf{F}_{-pq} &= \begin{bmatrix} F_{1x} & F_{1y} & F_{1z} & F_{2x} & \dots & F_{Nz} \end{bmatrix}_{-pq} \\ \boldsymbol{\sigma}_{-pq} &= \begin{bmatrix} \sigma_{11} & \sigma_{12} & \sigma_{13} & \sigma_{21} & \dots & \sigma_{33} \end{bmatrix}_{-pq}\end{aligned} \tag{30}$$

The mixed second derivatives with respect to cell and deformed coordinates become:

$$\frac{\partial^2 U_f}{\partial h_{pq}\,\partial \mathbf{d}} = \frac{\left[-\mathbf{F}_{+pq} \cdot (\mathbf{h}_0^{-1}\mathbf{h}_+)^T\right] - \left[-\mathbf{F}_{-pq} \cdot (\mathbf{h}_0^{-1}\mathbf{h}_-)^T\right]}{2\Delta h_{pq}} \tag{31}$$

where $\mathbf{h}_+$ and $\mathbf{h}_-$ denote the cells after positive and negative perturbations, respectively.

Finally, the mixed second derivatives with respect to cell coordinates are:

$$\frac{\partial^2 U_f}{\partial h_{pq}\,\partial \mathbf{h}} = \frac{\left[V\,\mathbf{h}_+^{-T}\boldsymbol{\sigma}_{+pq}\right] - \left[V\,\mathbf{h}_-^{-T}\boldsymbol{\sigma}_{-pq}\right]}{2\Delta h_{pq}} \tag{32}$$

### 2.1.4 Evaluation of the reference Gibbs free energy

Once the extended Hessian is constructed, the next step is to evaluate the reference Gibbs free energy. Its analytical expression is:

$$G_{\text{ref}}(P,T) = U_{f,0} - \frac{1}{\beta}\ln\left(\frac{1}{V_s V_0^N}\right) - \frac{3}{\beta}\ln\left(\prod_{i=1}^{N}\frac{1}{\lambda_i}\right) - \frac{1}{2\beta}\ln\left(\prod_{i=1}^{3N+3}\frac{2\pi}{\beta D_i}\right) \tag{33}$$

where $V_s$ is an arbitrary normalization volume, $V_0$ is the volume at the minimum of $U_f$, and $U_{f,0} = U_{\text{real},0} + PV_0 - \frac{N-2}{\beta}\ln(V_0)$ the minimum value of $U_f$. Further, $\lambda_i = \frac{h}{\sqrt{2\pi m_i k_B T}}$ is the thermal wavelength of atom $i$, and $D_i$ are the non-zero eigenvalues of the extended Hessian.

The variable $V_s$ should be the same for all simulations and was set equal to 1 Å$^3$, such that it drops out of the expression. The arguments of the second and third natural logarithm are a product of $3N$ or $3N+3$ terms, respectively, where the factors contain physical constants like the Boltzmann or Planck constant. These products might become incredibly small and cause numerical overflow. In order to guarantee numerical stability, the following expression was implemented:

$$\begin{aligned} G_{\text{ref}}(P,T) = U_{f,0} + \frac{N}{\beta}\ln\left(V_0\right) - \frac{3}{2\beta}\sum_{i=1}^{N}\ln(m_i) \\ - \frac{3N}{\beta}\ln\left(\frac{\sqrt{2\pi/\beta}}{h}\right) + \frac{1}{2\beta}\sum_{i=1}^{3N+3}\ln(D_i) - \frac{3N+3}{2\beta}\ln\left(\frac{2\pi}{\beta}\right) \end{aligned} \tag{34}$$

where the logarithm of the product is written as the sum of logarithms.

## 2.2 MD simulations in the NPT harmonic PES

The TI correction between our new reference PES and the real crystal at constant pressure is given by:

$$\int_0^1 \mathrm{d}\lambda \, \langle U_{\text{real}} - U_{\text{ref}} \rangle_{\lambda,P,T}. \tag{35}$$

For each $\lambda \in [0,1]$, the mixed PES is defined as:

$$\begin{aligned} U_{\text{mixed}}(\lambda) &= (1-\lambda)\,U_{\text{ref}} + \lambda\,U_{\text{real}} \\ &= (1-\lambda)\big(\mathcal{T}^2\left(U_f\right) - U_{\text{bias}}\big) + \lambda\,U_{\text{real}}. \end{aligned} \tag{36}$$

Sampling the mixed PES $U_{\text{mixed}}(\lambda)$ with isothermal-isobaric MD simulations allows us to evaluate the ensemble average $\langle U_{\text{real}} - U_{\text{ref}} \rangle_{\lambda,P,T}$ at a given $\lambda$. The integral over $\lambda$ is discretized using the trapezoidal rule. MD simulations using the real PES (in our case, the MACE MLIP[3]) and the bias PES (implemented through PLUMED[4]) require no additional development. However, MD simulations with the extended harmonic PES $\mathcal{T}^2(U_f)$ do require an implementation of the corresponding energy, forces, and stresses for a given input

geometry. As MD integration itself can be handled by i-PI,[7] only this evaluation step must be implemented, as described below.

**(i) Transformation of the input geometry to deformed coordinates; the cell remains unchanged.** The input geometry consists of Cartesian coordinates $\mathbf{r}_i$ of $N$ particles, collected in an $(N, 3)$ matrix, together with the cell matrix $\mathbf{h}$. The deformed coordinates $\mathbf{d}_i$ are defined as:

$$\mathbf{d}_i = \mathbf{r}_i \cdot \mathbf{h}^{-1}\mathbf{h}_0. \tag{37}$$

The deformed coordinates and cell matrix are then flattened (row-major convention) into a single vector $\mathbf{x}$:

$$\mathbf{x} = \begin{bmatrix} d_{1x} & d_{1y} & d_{1z} & d_{2x} & \cdots & d_{Nz} & h_{11} & h_{12} & \cdots & h_{33} \end{bmatrix}. \tag{38}$$

The optimized reference geometry defines an analogous vector $\mathbf{x}_0$.

**(ii) Evaluation of the harmonic energy, deformed forces, and cell gradient.** Let $\mathbf{H}_{\text{ext}}$ denote the extended Hessian and $U_{f,0}$ the energy of the optimized geometry. The harmonic energy is then:

$$\mathcal{T}^2(U_f)(\mathbf{x}) = U_{f,0} + \frac{1}{2}\begin{bmatrix}\mathbf{x} - \mathbf{x}_0\end{bmatrix} \cdot \mathbf{H}_{\text{ext}} \cdot \begin{bmatrix}\mathbf{x} - \mathbf{x}_0\end{bmatrix}^T. \tag{39}$$

Since the extended Hessian is symmetric, the gradient with respect to $\mathbf{x}$ is:

$$\nabla_{\mathbf{x}}\mathcal{T}^2(U_f) = \begin{bmatrix}\mathbf{x} - \mathbf{x}_0\end{bmatrix} \cdot \mathbf{H}_{\text{ext}}. \tag{40}$$

The first $3N$ components of $\nabla_{\mathbf{x}}\mathcal{T}^2(U_f)$ give the gradient with respect to the deformed coordinates, $\nabla_{\mathbf{d}}\mathcal{T}^2(U_f)$, while the final nine components define the cell gradient, $\nabla_{\mathbf{h}}\mathcal{T}^2(U_f)$.

**(iii) Back-transformation of deformed forces and the cell gradient to Cartesian forces and stresses.** MD simulations require Cartesian forces and the stress tensor. The $(1, 9)$ cell gradient $\nabla_{\mathbf{h}} U_f$ is reshaped into the $(3, 3)$ matrix $\frac{\partial U_f}{\partial \mathbf{h}}$. The stress tensor then follows as:[6]

$$\boldsymbol{\sigma} = \frac{1}{V} \cdot \mathbf{h}^T \cdot \frac{\partial U_f}{\partial \mathbf{h}}. \tag{41}$$

The Cartesian forces $\nabla_{\mathbf{r}_i} U_f$ are obtained via:

$$\nabla_{\mathbf{r}_i} U_f = \nabla_{\mathbf{d}_i} U_f \cdot (\mathbf{h}^{-1}\mathbf{h}_0)^T. \tag{42}$$

as was verified via a finite-difference scheme.

The complete pipeline of the new TI workflow is illustrated in figure 2.

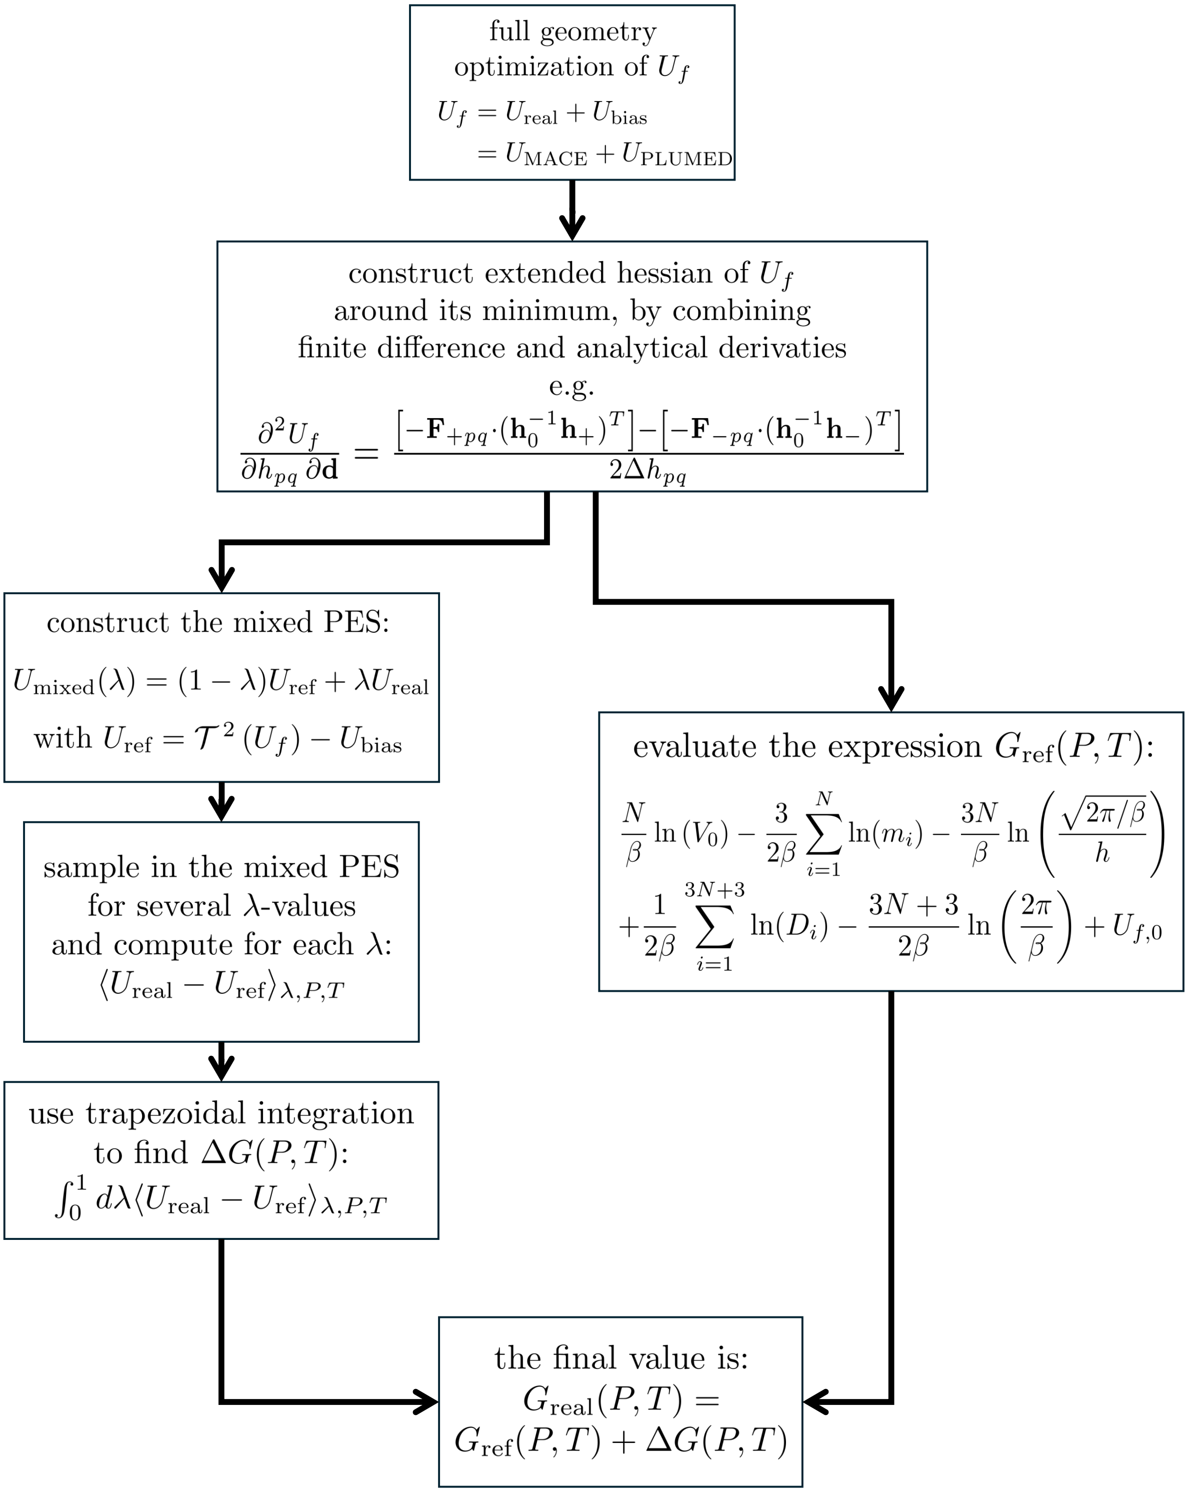


Figure 2: Technical overview of the workflow of the new TI scheme.

# 3 Computational details

## 3.1 MD settings

Independently on the material, temperature and pressure control were achieved using the Langevin thermostat[8] and the Martyna-Tobias-Tuckerman-Klein (MTTK) barostat,[9] respectively. All ice simulations employed a timestep of 0.5 fs, whereas the $CsPbI_3$ simulations used a timestep of 2 fs. For equilibration purposes, the first 4 000 steps were omitted for each ice MD simulation, whereas 20 000 steps were omitted for each $CsPbI_3$ MD simulation. Configurations were sampled every 200 steps and treated as uncorrelated.

**Ice workflow settings** For the conventional method, NPT MD simulations of $1e5$ steps were performed, and the average cell and the harmonic reference were computed. Subsequently, the anharmonic correction was computed via NVT-$\lambda$-TI via $1e5$ steps for 10 values of $\lambda \in [0, 1]$. For the new approach, the anharmonic correction was computed via NPT-$\lambda$-TI, using MD simulations of $1e5$ steps for each of the same 10 $\lambda$ values.

**$CsPbI_3$ workflow settings** When NVT REX MD or NPT REX MD was used, the temperatures were logarithmically spaced between the lowest one and 600 K, with replica-exchange attempts every 200 steps between every replica pair. At 300 K, there were 4 replicas; at 150 K, 8 replicas; at 75 K, 16.

For the conventional method, NPT equilibration was carried out using NPT REX MD. For all replicas, at least $4e5$ MD steps were performed. The harmonic Helmholtz free energy was evaluated at 600 K for all optimized structures. The NVT-$\lambda$-TI corrections were computed from MD simulations of $4e5$ steps for each of the 14 $\lambda$ values. Temperature corrections were obtained from NVT REX MD simulations, each simulated for $4e5$ MD steps.

For the new approach, a single NPT harmonic reference system was constructed at 600 K. The NPT-$\lambda$-TI correction was computed using MD simulations of $4e5$ steps for each of the 14 $\lambda$ values. Temperature corrections were obtained using the same NPT REX MD data

generated during the NPT equilibration step of the conventional workflow.

## 3.2 Computational cost for the $CsPbI_3$ case study

The total computational cost for the $CsPbI_3$ case study can be decomposed as summarized in Table 1.

Table 1: **Decomposition of the computational cost for the $CsPbI_3$ case study.** The cost of each step is reported as the product of the number of MD steps, and either the number of replicas or the number of $\lambda$ values (for temperature correction or anharmonic correction, respectively). The computational cost of the optimization and Hessian calculation are negligible and therefore not mentioned in the table.

| **Conventional method** | 75 K | 150 K | 300 K | 600 K |
|---|---|---|---|---|
| NPT equilibration | $10 \cdot 10^5 \times 16$ | $4 \cdot 10^5 \times 8$ | $4 \cdot 10^5 \times 4$ | $4 \cdot 10^5$ |
| NVT $\lambda$-TI (at 600 K) | $4 \cdot 10^5 \times 14$ | $4 \cdot 10^5 \times 14$ | $4 \cdot 10^5 \times 14$ | $4 \cdot 10^5 \times 14$ |
| NVT temperature TI | $4 \cdot 10^5 \times 16$ | $4 \cdot 10^5 \times 8$ | $4 \cdot 10^5 \times 4$ | $4 \cdot 10^5$ |
| **New method** | 75 K | 150 K | 300 K | 600 K |
| NPT $\lambda$-TI (at 600 K) | | | | $4 \cdot 10^5 \times 14$ |
| NPT temperature TI | $10 \cdot 10^5 \times 16$ | $4 \cdot 10^5 \times 8$ | $4 \cdot 10^5 \times 4$ | $4 \cdot 10^5$ |

At 600 K, the computational cost of the conventional and new approach is nearly identical, differing by only about 6% (15/16), and the associated statistical errors are also comparable. At lower temperatures, however, the conventional workflow appears substantially more expensive. This difference can be traced back to two key factors. First, in the conventional method the NVT $\lambda$-TI correction must be performed for four distinct average cells (one per envisioned temperature), whereas the flexible NPT reference in the new method allows a single NPT $\lambda$-TI calculation at high temperature. Second, the conventional approach requires two separate REX simulations: one for the temperature correction and one for the NVT-to-NPT correction, while the new method requires only the former.

As a result, the total computational effort per $CsPbI_3$ phase amounts to $268e5$ steps for the new method and $552e5$ for the conventional method. We want to stress that this does not mean that the new method is twice cheaper than the conventional one. Instead, it arises from

our choice to enforce a strictly independent and methodologically symmetric comparison, in which the NVT-to-NPT correction is treated as the final step of the conventional workflow. In practical applications, a cost-minimizing implementation of the conventional method would instead perform the NVT-to-NPT correction only once at 600 K and subsequently apply all temperature corrections in the NPT ensemble.

This observation is further clarified by considering the schematic comparison in Fig. 1 of the main manuscript. In both workflows, the first step is a $\lambda$-TI calculation, which has a very similar computational cost and statistical uncertainty, independently if it is an NVT or NPT correction. Also, the final step of both workflows, namely the temperature correction, is identical. The only additional contribution specific to the conventional approach is therefore the NVT-to-NPT correction, which is comparatively rather inexpensive.

We thus conclude that - provided temperature corrections are performed in the NPT ensemble - the conventional and new method exhibit a very similar computational cost.

# 4 MLIP generation

The training scripts and datasets are available upon request.

## 4.1 Ice

A MLIP based on the MACE architecture[10,11] and capable of describing multiple ice phases was trained from scratch. As reference level of theory, we selected revPBE-D3(BJ) / MOLOPT-TZV2P[12–15] as implemented in CP2K 2024.1,[16] due to its good computational efficiency and known ability of describing the structure of liquid water.[17] A cutoff of 1000 Ry was selected for the complementary plane-waves basis set[18] of CP2K and GTH pseudopotentials[19] were used to smooth the electron density around the atomic nuclei.

As initial dataset, we selected the structures of the ice phases found in the experimental phase diagram[20] (Ic, Ih, II, III, IV, V, VI, VII, VIII, IX, X, XI, XII, XIII, XIV, XV, XVI, XVI, XVII, XVIII, XIX) and, for each, use the atomic simulation environment[2] (ASE) to construct a supercell such that all cell lengths are within 12 and 20 Å and as close to orthorhombic as possible. In this way, the sampling of the Brillouin zone can be restricted to the gamma point. We then implemented an algorithm that first scrambles the H atoms between water molecules (potentially leading more or less than 2 H atoms to be bonded to an O atom) and, subsequently, reshuffles them to ensure that each O is linked to two H atoms. This allows to randomly generate proton-disordered structures - giving additional flexibility to the model. The procedure was repeated 8 times per phase with additional rattling of the atomic coordinates. The structures generated in this way were added to the liquid water dataset of Cheng et al.[21] and the whole dataset evaluated with the target level of theory.

Such initial dataset of 1,753 structures was randomly split 90:10 into a training and validation sets, which were then used to train an initial MACE model. The most relevant hyperparameters are listed in Tab. 2. To expand the dataset and improve its robustness, we picked the 8 structures of each phase (plus 8 additional structures for liquid water)

and attribute them a pressure beyond the border of their expected experimental stability range. For example, for ice Ih, we selected 8 pressures equally spaced in logarithmic space between $10^{-10}$ and 1 GPa. In addition, each structure was duplicated 8 times and attributed a temperature linearly spaced between 50 and 400 K. All structures were then propagated in the NPT ensemble at the selected conditions for 5 ps, for a total of 22 (21 ice phases + liquid water) $\times$ 8 (pressures) $\times$ 8 (temperatures) = 1,408 molecular dynamics simulations. Of these, 1,188 proved to be stable and, therefore, the final snapshot was extracted, evaluated with CP2K, and added to the training set.

Table 2: The hyperparameters for the MLIP model of water and $CsPbI_3$. All other hyperparameters were kept at their default values.

| **Hyperparameter** | **Ice** | $\mathbf{CsPbI_3}$ |
|---|---|---|
| `r_max` | 6.5 Å | 7.0 Å |
| `num_channels` | 64 | 16 |
| `energy_weight` | 100 | 10 |
| `batch_size` | 8 | 2 |
| `num_radial_basis` | 16 | 8 |
| `patience` | 20 | 30 |
| `max_num_epochs` | 1000 | 400 |
| `swa` | `True` | `False` |
| `start_swa` | 500 | / |
| `swa_energy_weight` | 200 | / |
| `correlation` | 3 | 4 |
| `ema` | `False` | `True` |

With this final dataset of 2,899 structures labeled with DFT energy and forces, we trained a final MACE MLIP which achieved final root mean squared errors of 1.5 and 1.0 meV per atom on the energies of the training and validation sets, respectively, and 45.5 and 50.8 meV·Å$^{-1}$ on the forces of the training and validation sets, respectively. This model proved to be stable for all the production TI simulations and, because we do not aim at reaching perfect accuracy in the description of the potential energy surface, no further tests on the model accuracy were performed.

## 4.2 $CsPbI_3$

We generated a dataset comprising 90 distinct polymorphs of $CsPbI_3$, including both the black and yellow phases, as well as a diverse set of intermediate structures that may form along the transition pathway between these phases. This dataset therefore spans a wide variety of local atomic environments. For each structure, MD simulations were performed using the foundation model MACE-MP-0[?] at temperatures of 150 K and 600 K. Both NVT and NPT simulations were carried out, with the latter performed at a pressure of 0.1 MPa.

The resulting trajectories were subsampled to construct a database of 865 representative configurations. Energies and forces for these configurations were subsequently computed using DFT with the PBE-D3(BJ) XC functional as implemented in VASP.[?,?] This level of theory offers a favorable balance between accuracy and computational efficiency for $CsPbI_3$.[22,?] Projector-augmented-wave (PAW) potentials[?] were employed with the following valence electron configurations: Cs_sv ($5s^2 5p^6 6s^1$), Pb_d ($5d^{10} 6s^2 6p^2$), and I ($5s^2 5p^5$). All calculations used a Γ-centered $1 \times 1 \times 1$ k-point grid and a plane-wave cutoff energy of 500 eV.

The MLIP was trained on this dataset using the MACE architecture,[3] as implemented in the psiflow framework.[6] Several hyperparameters were modified relative to the default MACE settings, as detailed in Tab. 2. After approximately 9 hours of training on an AMD MI250x GPU, the resulting model achieved validation errors of 1.0 meV per atom for energies and 32.7 meV/Å for forces.

# 5 Visualization of tilted cell configurations

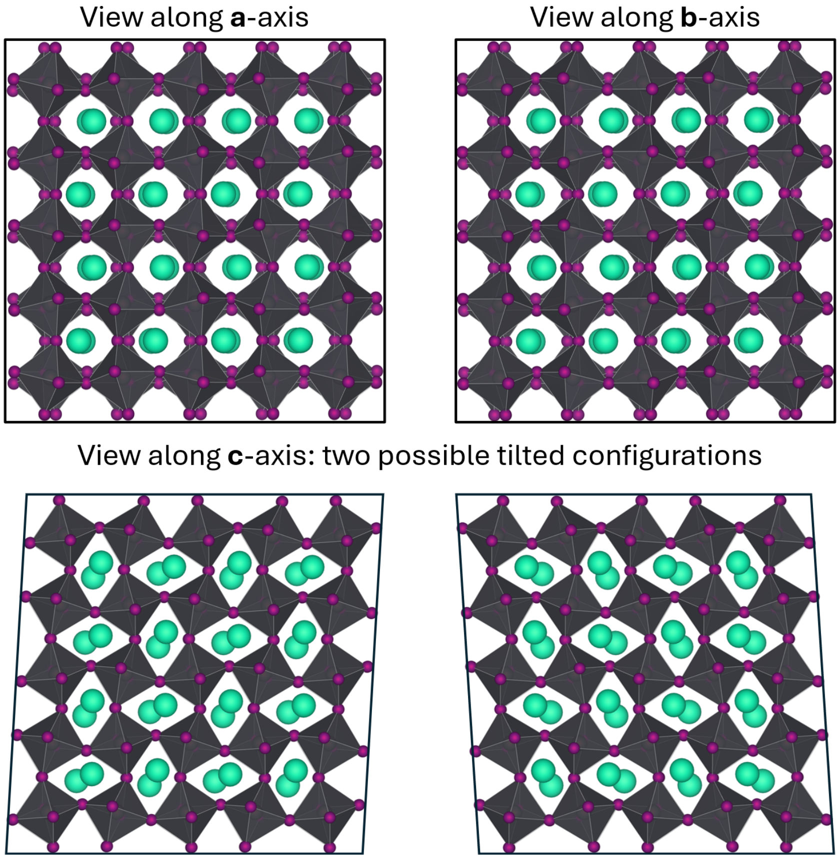


Figure 3: Visualization of tilted cell configurations. While two out of three cell angles are 90°, the third angle is either 87° or 93°, leading to two degenerate cell minima illustrated in the figure. As the three cell angles (or three cell vectors) are interchangeable, this leads to a total of six degenerate cell minima. For each of these six cell minima, four degenerate configurations of the octahedra are possible, yielding a total of 24 degenerate geometric minima.[22]

# References


(1) Tuckerman, M. E. *Statistical Mechanics: Theory and Molecular Simulation*, 2nd ed.; Oxford University Press: Oxford, 2010.

(2) Larsen, A. H.; Mortensen, J. J.; Blomqvist, J.; others The atomic simulation environment — a Python library for working with atoms. *Journal of Physics: Condensed Matter* **2017**, *29*, 273002.

(3) Batatia, I.; Kovács, D. P.; Simm, G. N. C.; Ortner, C.; Csányi, G. MACE: Higher order equivariant message passing neural networks for fast and accurate force fields. 2023.

(4) PLUMED Consortium Promoting transparency and reproducibility in enhanced molecular simulations. *Nature Methods* **2019**, *16*, 670–673.

(5) Baydin, A. G.; Pearlmutter, B. A.; Radul, A. A.; Siskind, J. M. Automatic differentiation in machine learning: A survey. *Journal of Machine Learning Research* **2018**, *18*, 1–43.

(6) Vandenhaute, S.; Cools-Ceuppens, M.; DeKeyser, S.; Verstraelen, T. Machine learning potentials for metal-organic frameworks using an incremental learning approach. *npj Computational Materials* **2023**, *9*, 19.

(7) Litman, Y. et al. i-PI 3.0: A flexible and efficient framework for advanced atomistic simulations. *Journal of Chemical Physics* **2024**, *161*, 062504.

(8) Langevin, P. Sur la théorie du mouvement brownien. *Comptes Rendus de l'Académie des Sciences* **1908**, *146*, 530–533.

(9) Martyna, G. J.; Tuckerman, M. E.; Tobias, D. J.; Klein, M. L. Explicit reversible integrators for extended systems dynamics. *Molecular Physics* **1996**, *87*, 1117–1157.

(10) Batatia, I.; Kovacs, D. P.; Simm, G. N. C.; Ortner, C.; Csanyi, G. MACE: Higher order equivariant message passing neural networks for fast and accurate force fields. Advances in Neural Information Processing Systems. 2022.

(11) Batatia, I.; Batzner, S.; Kovács, D. P.; Musaelian, A.; Simm, G. N. C.; Drautz, R.; Ortner, C.; Kozinsky, B.; Csányi, G. The design space of E(3)-equivariant atom-centred interatomic potentials. *Nature Machine Intelligence* **2025**, *7*, 56–67.

(12) Perdew, J. P.; Burke, K.; Ernzerhof, M. Generalized gradient approximation made simple. *Physical Review Letters* **1996**, *77*, 3865–3868.

(13) Zhang, Y.; Yang, W. Comment on "generalized gradient approximation made simple". *Physical Review Letters* **1998**, *80*, 890–890.

(14) Grimme, S.; Antony, J.; Ehrlich, S.; Krieg, H. A consistent and accurate ab initio parametrization of density functional dispersion correction (DFT-D) for the 94 elements H–Pu. *Journal of Chemical Physics* **2010**, *132*.

(15) Grimme, S.; Ehrlich, S.; Goerigk, L. Effect of the damping function in dispersion corrected density functional theory. *Journal of Computational Chemistry* **2011**, *32*, 1456–1465.

(16) Kühne, T. D.; Iannuzzi, M.; Del Ben, M.; others CP2K: An electronic structure and molecular dynamics software package—Quickstep: Efficient and accurate electronic structure calculations. *Journal of Chemical Physics* **2020**, *152*.

(17) Pestana, L. R.; Mardirossian, N.; Head-Gordon, M.; Head-Gordon, T. Ab initio molecular dynamics simulations of liquid water using high quality meta-GGA functionals. *Chemical Science* **2017**, *8*, 3554–3565.

(18) VandeVondele, J.; Krack, M.; Mohamed, F.; Parrinello, M.; Chassaing, T.; Hutter, J.

Quickstep: Fast and accurate density functional calculations using a mixed Gaussian and plane waves approach. *Computer Physics Communications* **2005**, *167*, 103–128.

(19) Goedecker, S.; Teter, M.; Hutter, J. Separable dual-space Gaussian pseudopotentials. *Physical Review B* **1996**, *54*, 1703.

(20) Hansen, T. C. The everlasting hunt for new ice phases. *Nature Communications* **2021**, *12*, 3161.

(21) Cheng, B.; Engel, E. A.; Behler, J.; Dellago, C.; Ceriotti, M. Ab initio thermodynamics of liquid and solid water. *Proceedings of the National Academy of Sciences* **2019**, *116*, 1110–1115.

(22) Braeckevelt, T.; Goeminne, R.; Vandenhaute, S.; Borgmans, S.; Verstraelen, T.; Steele, J. A.; Roeffaers, M. B. J.; Hofkens, J.; Rogge, S. M. J.; Van Speybroeck, V. Accurately determining the phase transition temperature of $CsPbI_3$ via random-phase approximation calculations and phase-transferable machine learning potentials. *Chemistry of Materials* **2022**, *34*, 8561–8576.
